# Supplementary material for: FeedLens: Polymorphic Lenses for Personalizing Exploratory Search over Knowledge Graphs
Source: arXiv:2208.07531 ancillary file (2022-08-16)
Supplement: Supplementary file 1 [file Supplementary.pdf]

## 1 PILOT STUDIES

We conducted two pilot surveys to finalize the design of our exploratory search experience for papers and authors, using people's research feeds as lenses to define relevant content. Recall that research feeds are paper recommenders curated and maintained by a user for a particular topic or theme. We designed mock-ups for how to visualize lens (research feed) summaries of entities (papers and authors). Our mock-ups follow design principles for interactive systems, including ease of access to all types of information, features that have clear signifiers and affordances, overall ease of use, and user control over the information that is collected and included in features [2–4].

### 1.1 Design Survey 1: Semantic Scholar System Designers and Researchers

We conducted a survey ($n = 17$) to get initial feedback on our mock-ups from system designers and researchers who work on a popular scientific literature navigation tool, Semantic Scholar. By limiting this first design survey to people who work on Semantic Scholar, we were able to constrain our mock-ups for follow-up surveys and system design to ones that could feasibly be added to Semantic Scholar. Participants were presented with a total of 10 mock-ups, five for an author overview feature which would describe the relevance of an author based on lenses (see Figure 1 for some examples) and another five for a paper overview feature for the same purpose (see Figures 2–3 for some examples). Participants were asked to rank these mock-ups based on their preferences and (optionally) explain their ranking. We filtered and updated our mock-ups based on this initial feedback.

### 1.2 Design Survey 2: Semantic Scholar Users

Next, we conducted a survey with users who had created and continued to maintain research feeds on Semantic Scholar ($n = 13$). Participants were presented with seven mock-ups for paper overview and two for author overview (see Figures 2–3 for some examples). The survey included two sets of questions: (1) this-or-that questions which presented the designs in a decision-tree format, also intended to help participants get familiarized with the mock-ups; (2) a ranking question where participants provided their top-2 ranked visualizations and (optionally) explained their ranking.

### 1.3 Results: Design Guidelines

An inductive thematic analysis—conducted as open coding followed by axial coding [1]—of the open-ended responses from the survey resulted in the following guidelines based on people's explanations for their rankings. First, when displaying information for multiple types of entities at the same time, balancing informativeness and (visual) information overload is critical. Participants noted their preference for visualizations that supported quick perusal of information. Second, the new relevance information must be embedded in the existing interface design and not distract from information already on the page (for example, note the differences between the two designs in Figure 3). Finally, while quick perusal of relevance was critical, participants also wanted the option to dig deeper if they were so inclined. As such, mock-ups with signals or additional information that would help build trust in the relevance information were preferred (e.g., Design A indicates whether a paper is relevant to a lens using the existence of a colored square, but also presents the specific relevance value next to the square).

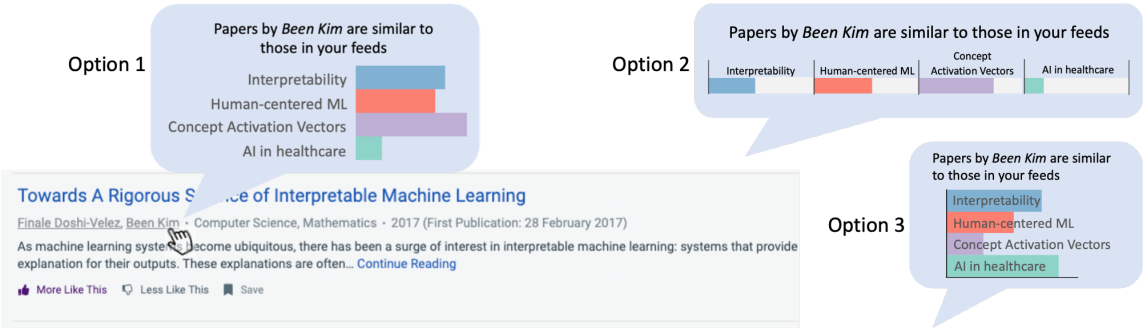


Fig. 1. Design mock-ups for author relevance overview showing the percentage of papers written by the author that are relevant to each of the user's feeds (i.e., lenses) in three different ways.

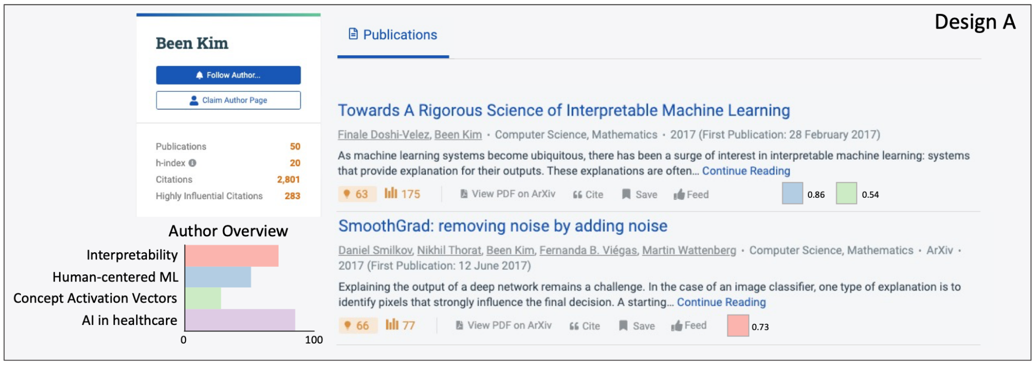


Fig. 2. Design mock-up for author and paper relevance presented on an author homepage. Author overview (bottom left) shows the percentage of papers written by the author that are relevant to each of the user's feeds. Paper relevance is indicated using numerical values in the range of 0–1, with squares representing the color of the user's corresponding feeds (colors are column-aligned for easy scanning, which explains different horizontal offsets).

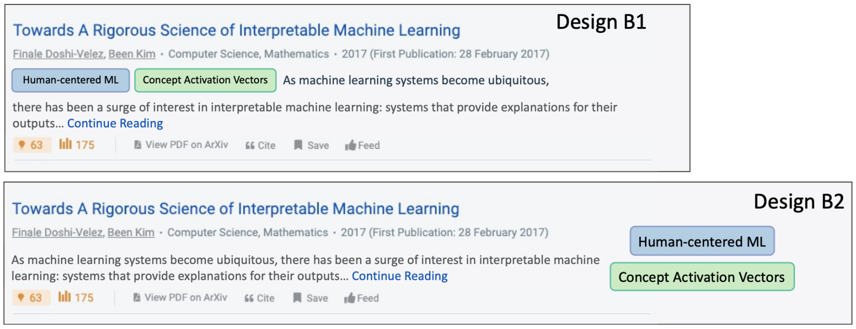


Fig. 3. Design mock-ups for paper relevance presented using a tag-based interface—if an author is relevant, the corresponding lens is added as a tag. Design B1 embeds these tags within a paper row; Design B2 displays them in the space to the right of a paper row. People prefer Design B1 since it is embedded in the existing interface.

### 1.4 Results: Design Preferences

There was no clear majority among our participants for any particular design mock-up, analyzed using the ranking question. Design B1 ($n = 4$) and Design A ($n = 3$) were most frequently ranked the best by our participants (Figures 3 and 2, respectively). The remaining votes were equally spread among the other mock-ups. We picked bar charts for the author overview visualization since both Designs A and B1 presented author overview this way. However, the paper overviews differ between the two designs. Given this lack of clear majority based on ranking, we analyzed participants' responses to the this–or–that questions for any preferences between Design A and B1 for paper overview visualization, once again noting no clear majority—Design A received marginally more "this" votes. We ultimately selected Design A for paper overview visualization since it met more design considerations from the open-text responses included by participants.

## 2 ALL COMPARISONS

| | | FeedLens | | Semantic Scholar | | |
|---|---|---|---|---|---|---|
| | | **Mean** | **Standard Deviation** | **Mean** | **Standard Deviation** | **p-value** |
| **Paper** | Diversity | 0.76 | 0.03 | 0.76 | 0.05 | 0.84 |
| | Novelty | 0.40 | 0.06 | 0.40 | 0.05 | 0.65 |
| | Relevance | 0.90 | 0.32 | 0.88 | 0.31 | 0.90 |
| | Obviousness | 0.29 | 0.29 | 0.71 | 0.29 | 0.05 |
| | Relevance - Subjective | 4.12 | 0.69 | 4.34 | 0.60 | 0.27 |
| | Novelty - Subjective | 4.48 | 0.49 | 4.23 | 0.67 | 0.04 |
| **Author** | Diversity | 0.55 | 0.25 | 0.56 | 0.26 | 0.70 |
| | Novelty | 0.51 | 0.18 | 0.48 | 0.17 | 0.13 |
| | Relevance - number of relevant papers | 13.00 | 7.75 | 6.20 | 9.39 | 0.92 |
| | Relevance - proportion of relevant papers | 24.50 | 10.50 | 10.50 | 12.22 | 0.94 |
| | Obviousness | 0.45 | 0.26 | 0.45 | 0.28 | 0.55 |
| | Relevance - Subjective | 3.95 | 0.75 | 3.82 | 0.75 | 0.63 |
| | Novelty - Subjective | 4.16 | 3.88 | 0.65 | 0.89 | 0.07 |

Table 1. Comparisons for all metrics calculated based on the final papers and authors selected for the literature review task. There were only marginal differences between FeedLens and Semantic Scholar for these metrics.

## REFERENCES


[1] Juliet M Corbin and Anselm Strauss. 1990. Grounded theory research: Procedures, canons, and evaluative criteria. *Qualitative sociology* 13, 1 (1990), 3–21.

[2] Don Norman. 2013. *The design of everyday things: Revised and expanded edition.* Basic books.

[3] Jef Raskin. 2000. *The humane interface: new directions for designing interactive systems.* Addison-Wesley Professional.

[4] Ben Shneiderman. 2003. The eyes have it: A task by data type taxonomy for information visualizations. In *The craft of information visualization.* Elsevier, 364–371.
